# Supplementary material for: EgoLive: A Large-Scale Egocentric Dataset from Real-World Human Tasks
Source: arXiv:2604.23570 source file (2026-04-26)
Supplement: Supplementary file 1 [file appendix.tex]

\newpage
\beginappendix

\section{Details   of tools}
\label{app:tools}
